# Supplementary material for: Compressibility of Distributed Document Representations
Source: arXiv:2110.07595 source file (2021-10-14)
Supplement: Supplementary file 1 [file appendix.tex]

\section{Classification performance}
The overall performance across all data sets is shown in Figures~\ref{fig:overalld2v}. Here, it can be observed that different compression mechanisms behave differently, however the consistent performance of \textsc{PCA}-based representations and the \textsc{CoRe}-ones can also be observed (e.g., the rightmost 4 data sets).
\begin{figure*}[h!]
    \centering
    \subfigure[Representation = DistilBERT]{
    \includegraphics[width=0.47\textwidth]{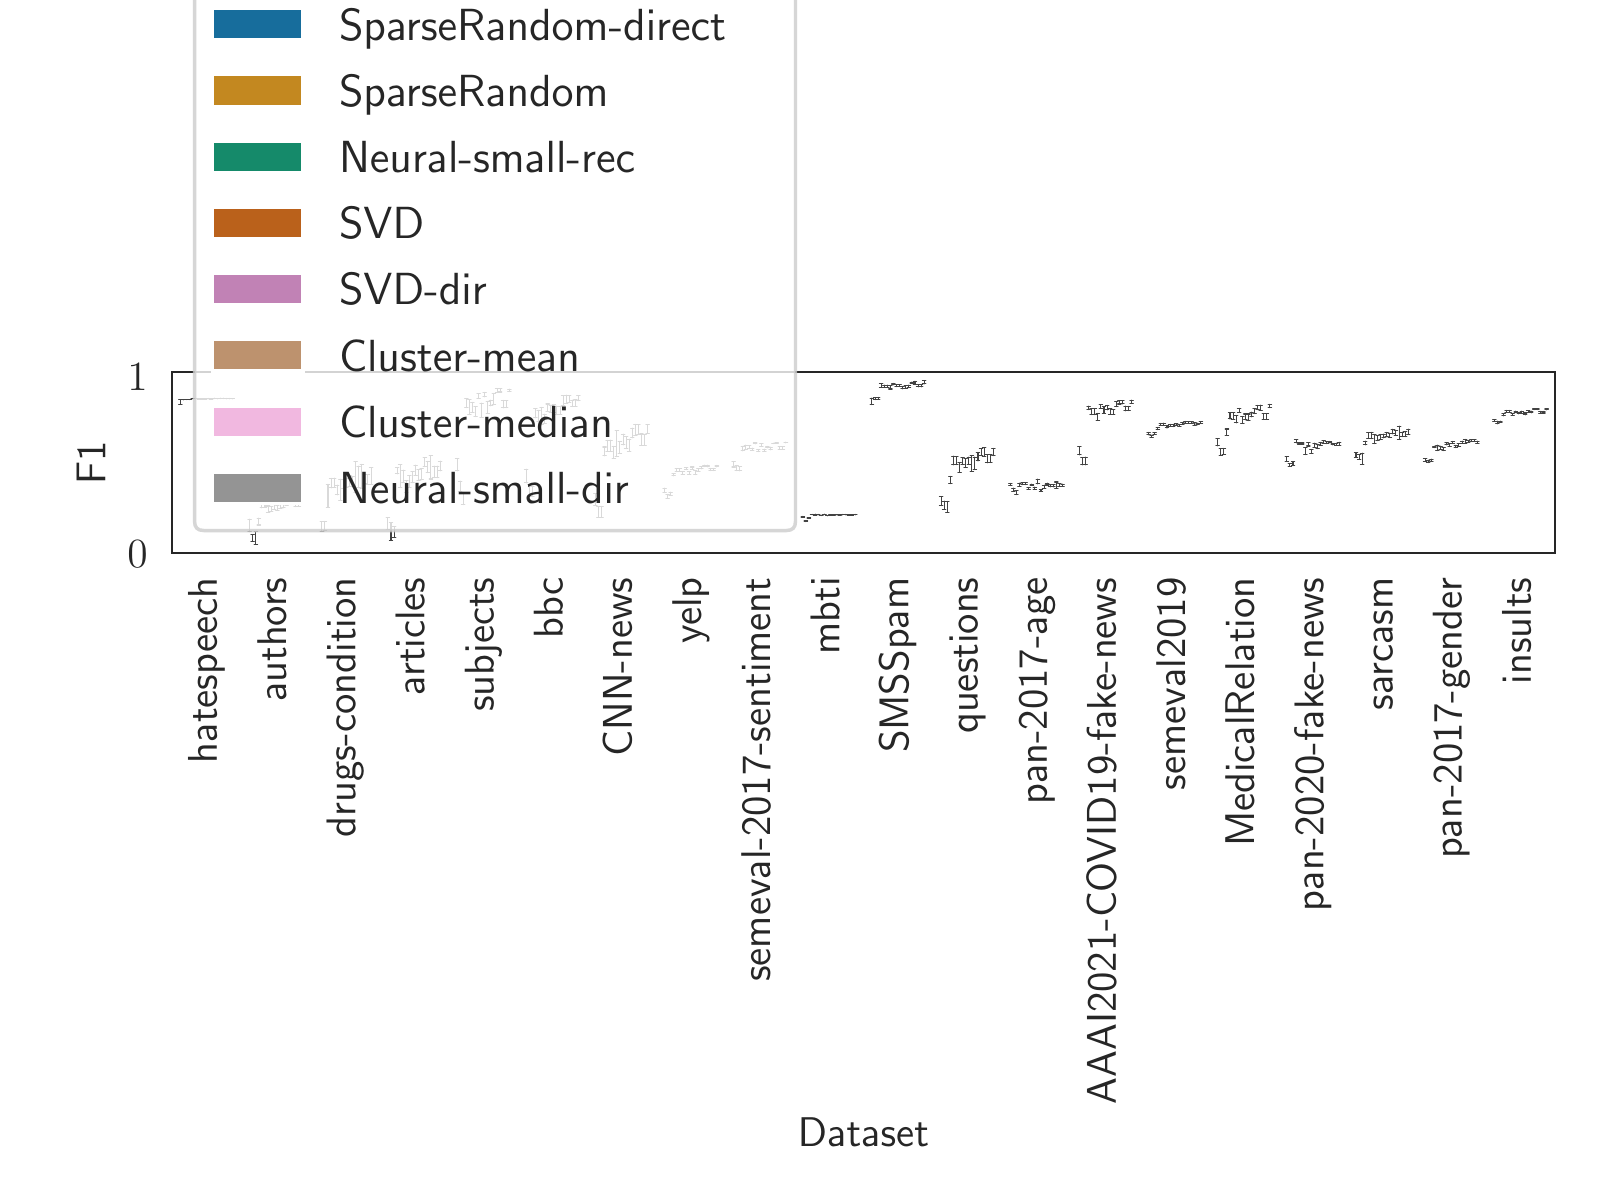}}
    \subfigure[Representation = doc2vec]{
    \includegraphics[width=0.47\textwidth]{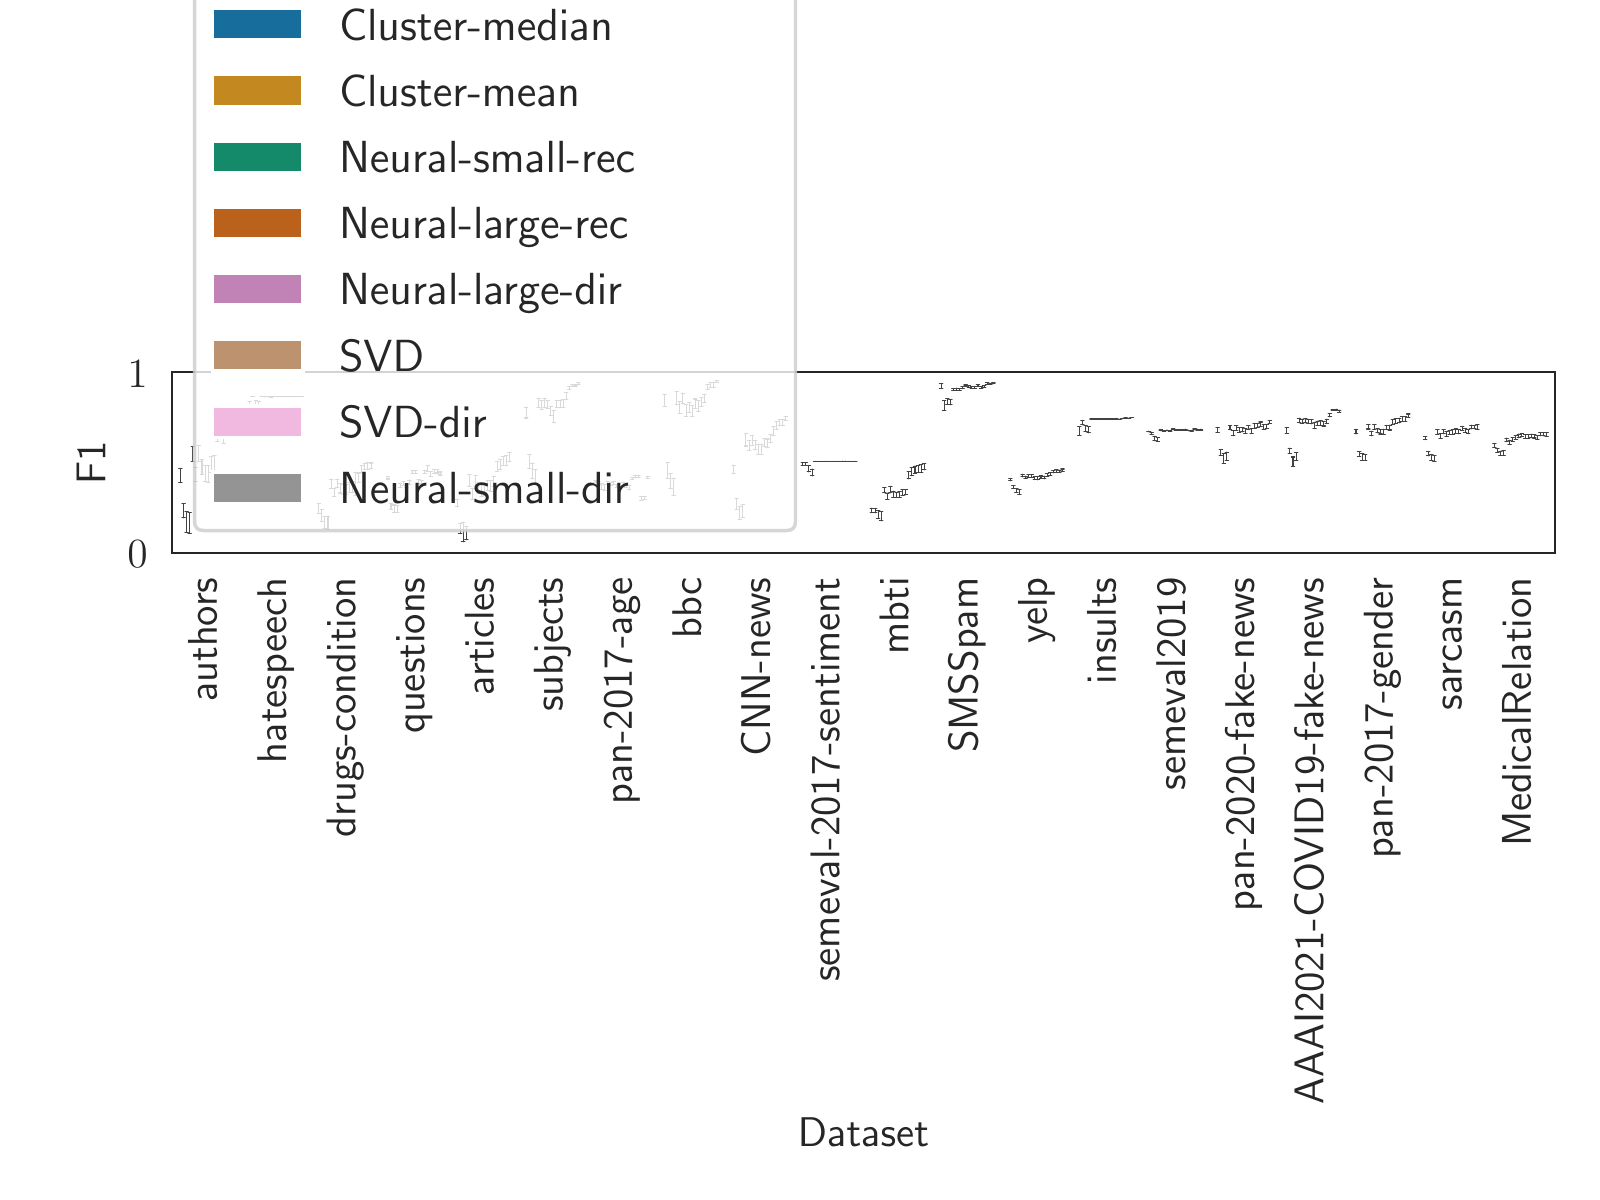}}
    \caption{Representation performances across different data sets. It can be observed that the performance of different compression mechanisms behaves similarly at individual data set level, however varies to large extent when compared across the data sets. The \emph{SMSSpam} data set, where the final classifier performs very well is also the data set which could be compressed the most whilst maintaining the performance.}
    \label{fig:overalld2v}
\end{figure*}
\section{Statistical analysis of compression performances. }
Finally, we present the critical distance diagrams~\cite{demvsar2006statistical} showing raking of representation-compressor pairs for two and three compression steps, respectively (Figure~\ref{fig:cd}).
\begin{figure*}[htb!]
\centering
\subfigure[$\tau = 2$]{
    \includegraphics[width=0.45\textwidth]{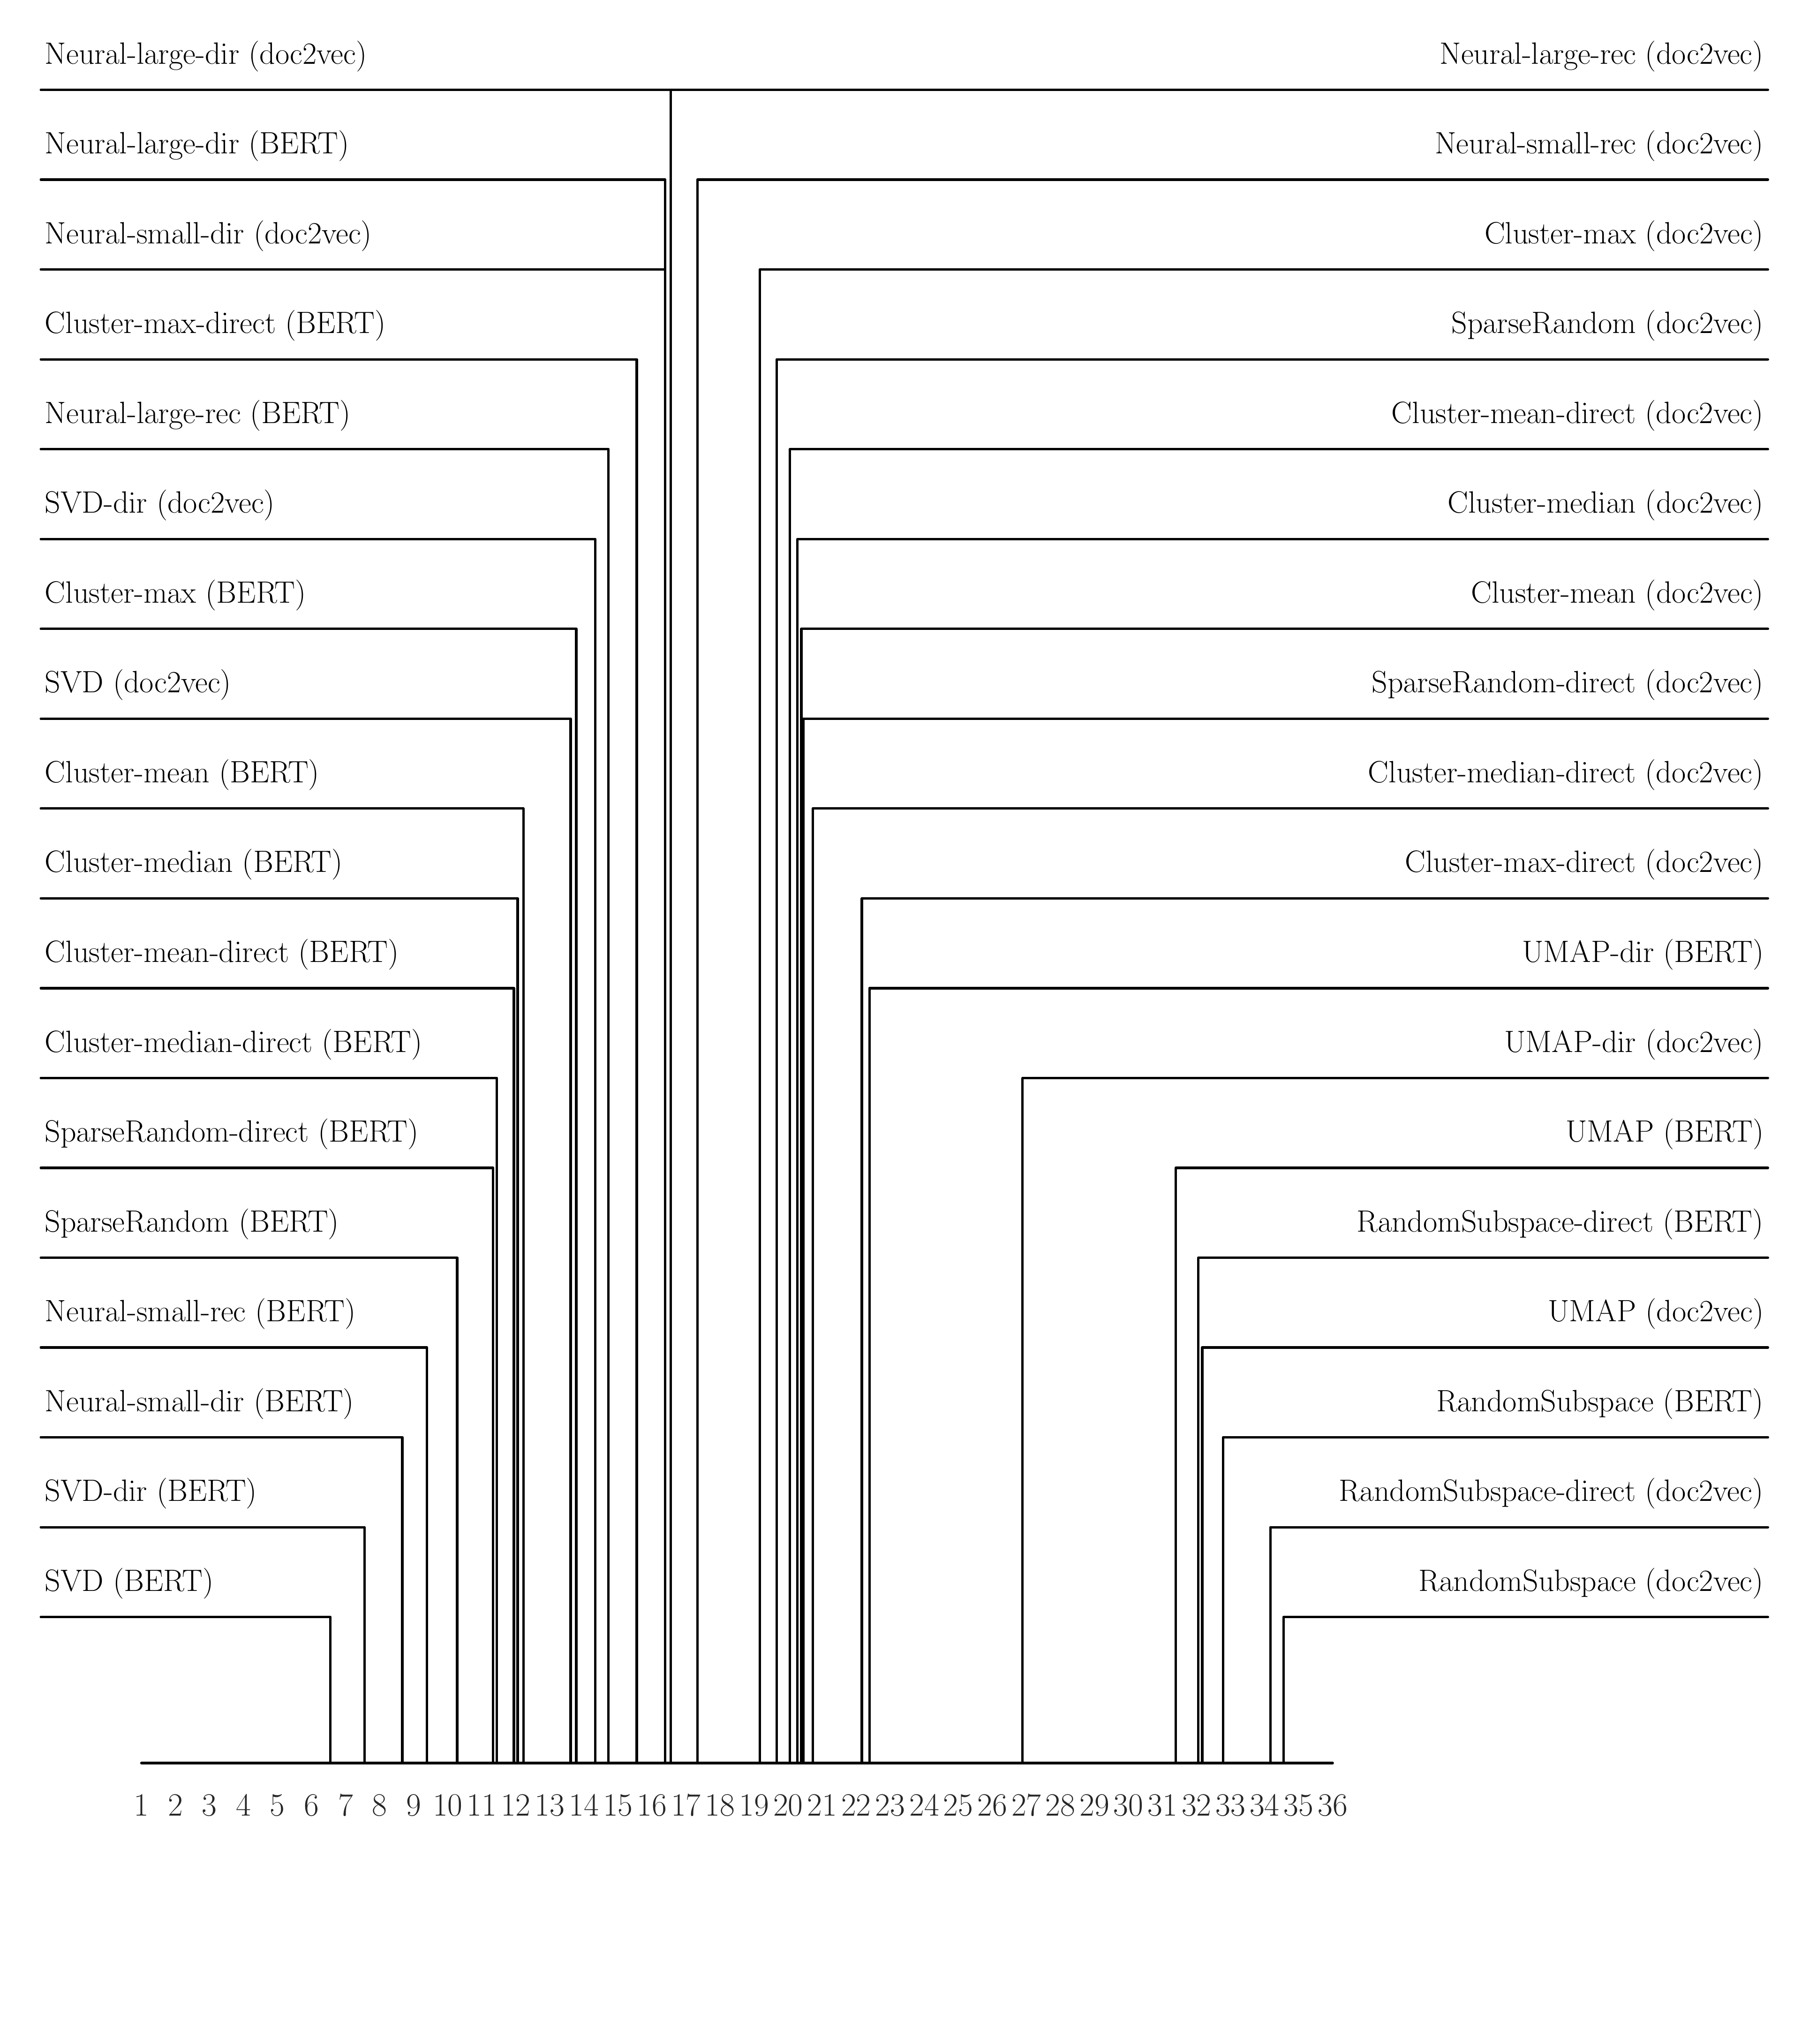}}
\subfigure[$\tau = 3$]{
    \includegraphics[width=0.45\textwidth]{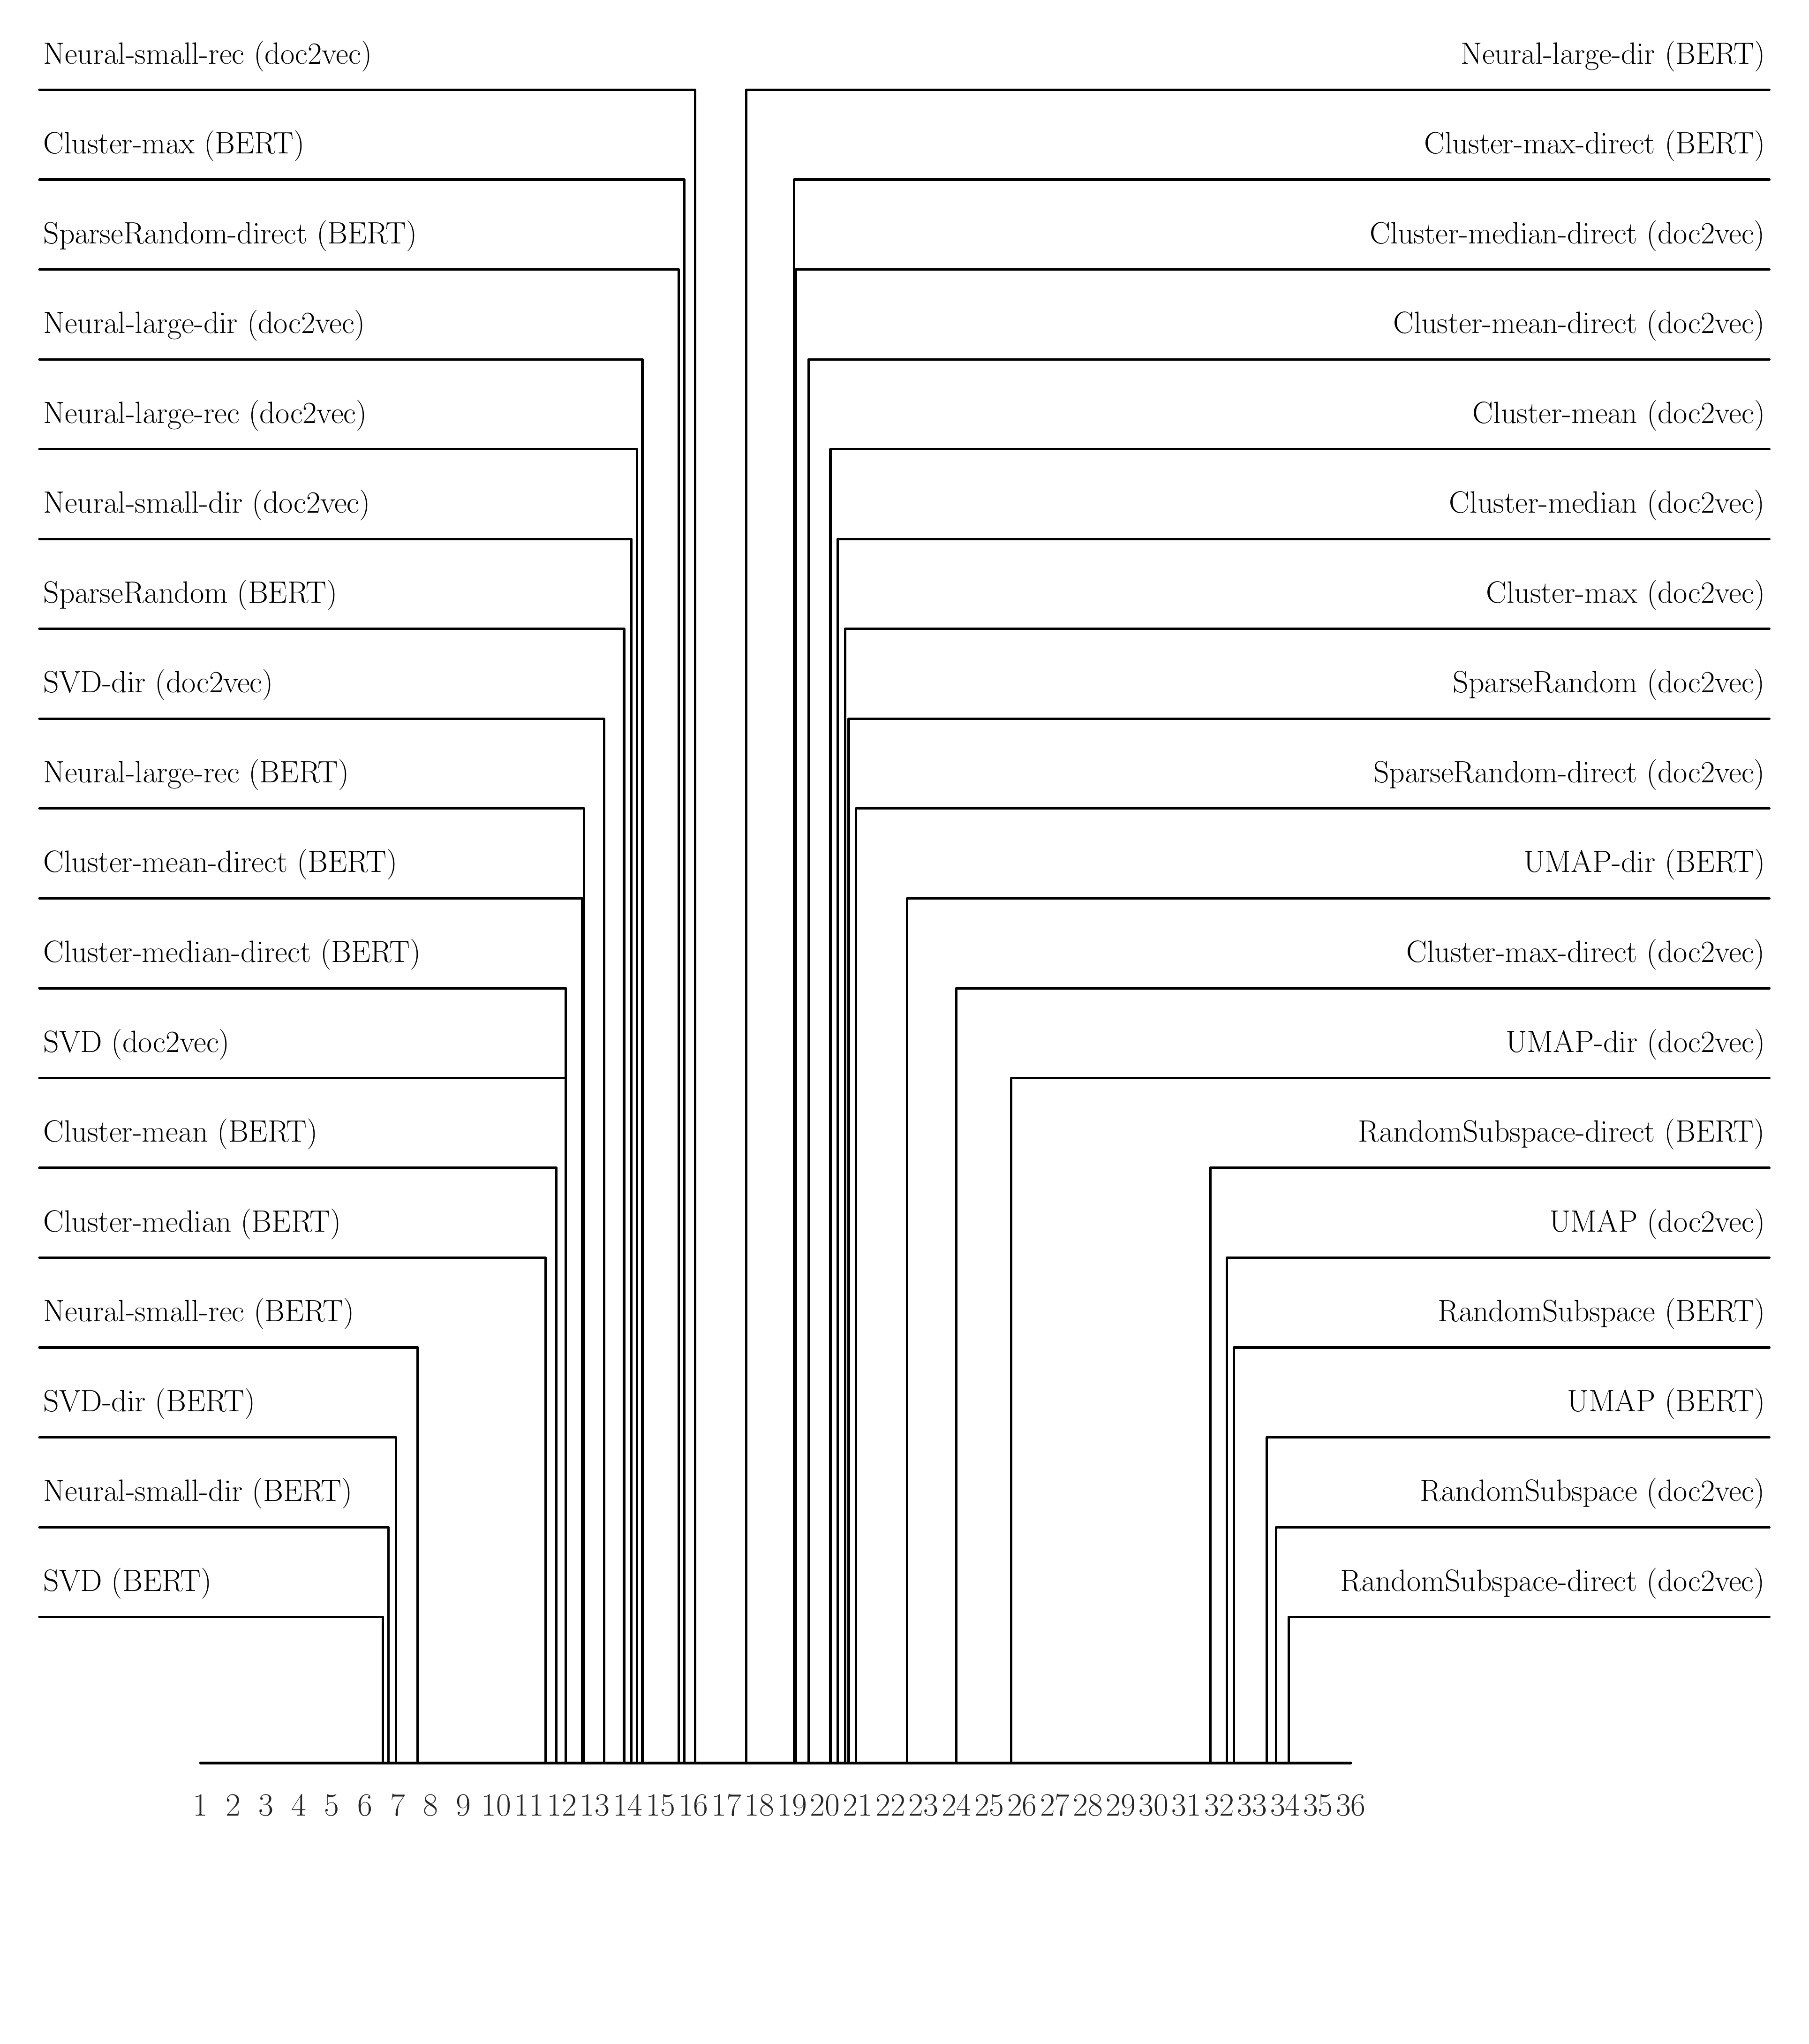}}
\subfigure[$\tau = 4$]{
    \includegraphics[width=0.45\textwidth]{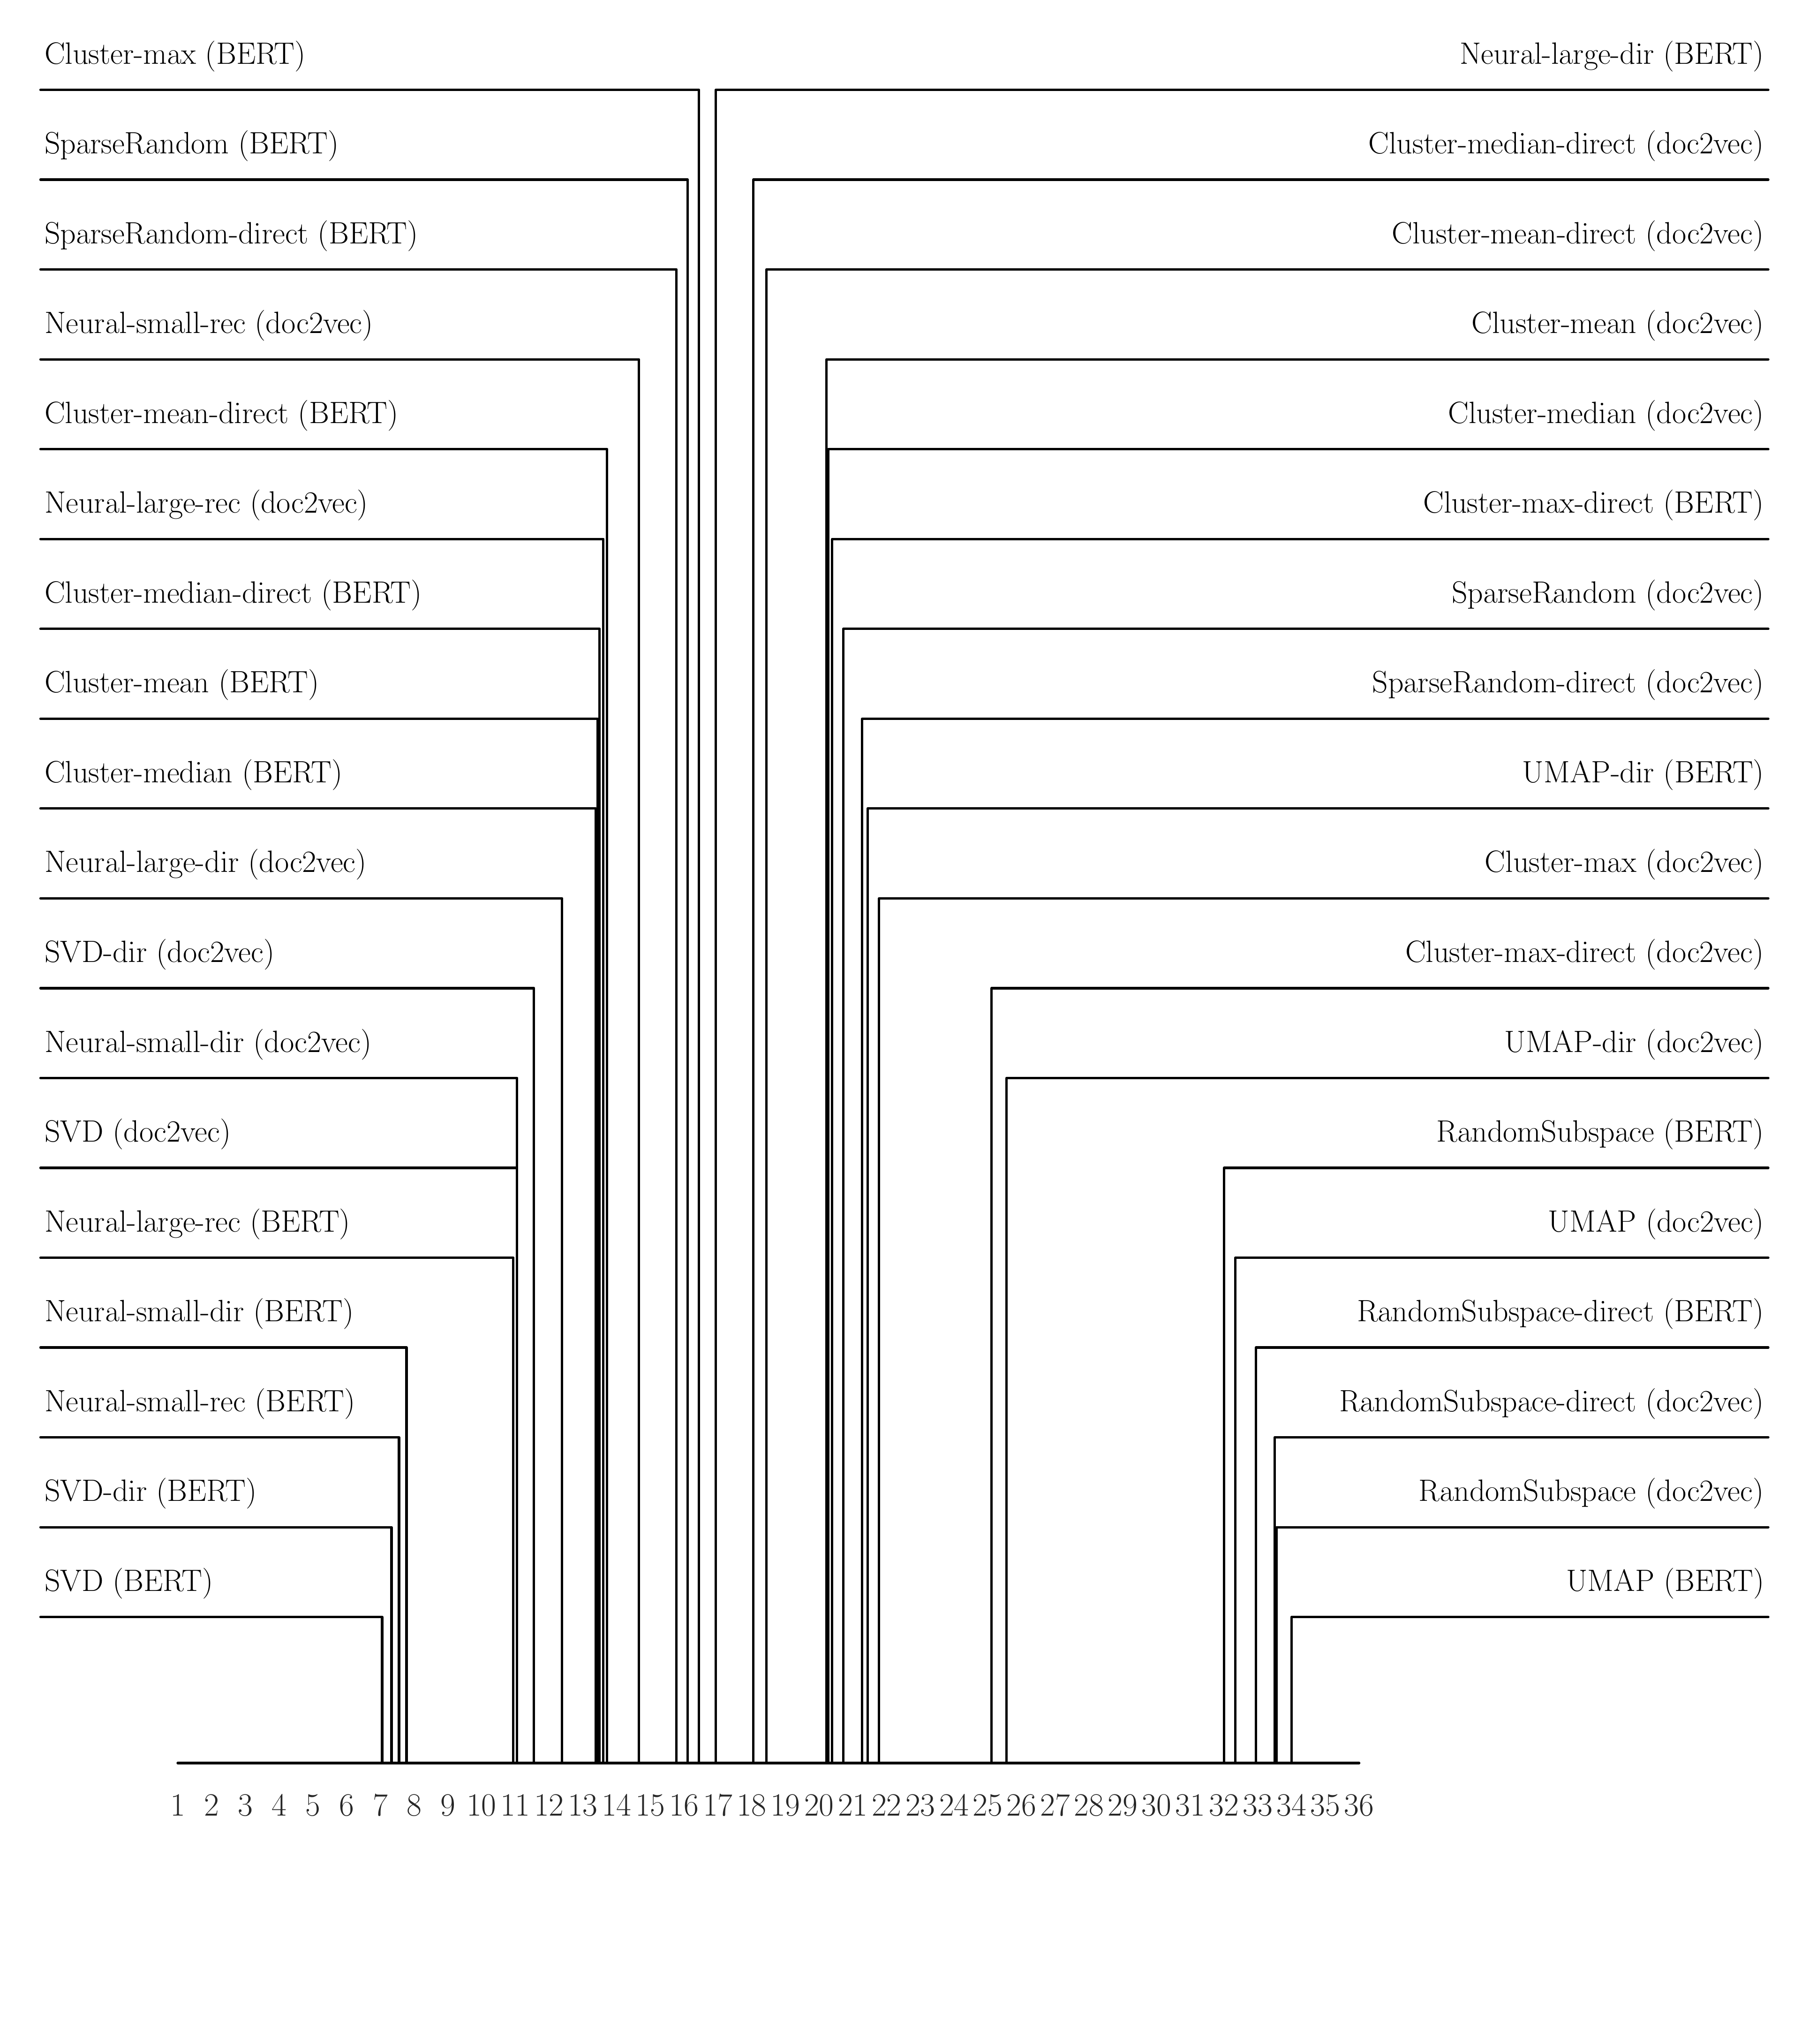}}
\subfigure[$\tau = 5$]{
    \includegraphics[width=0.45\textwidth]{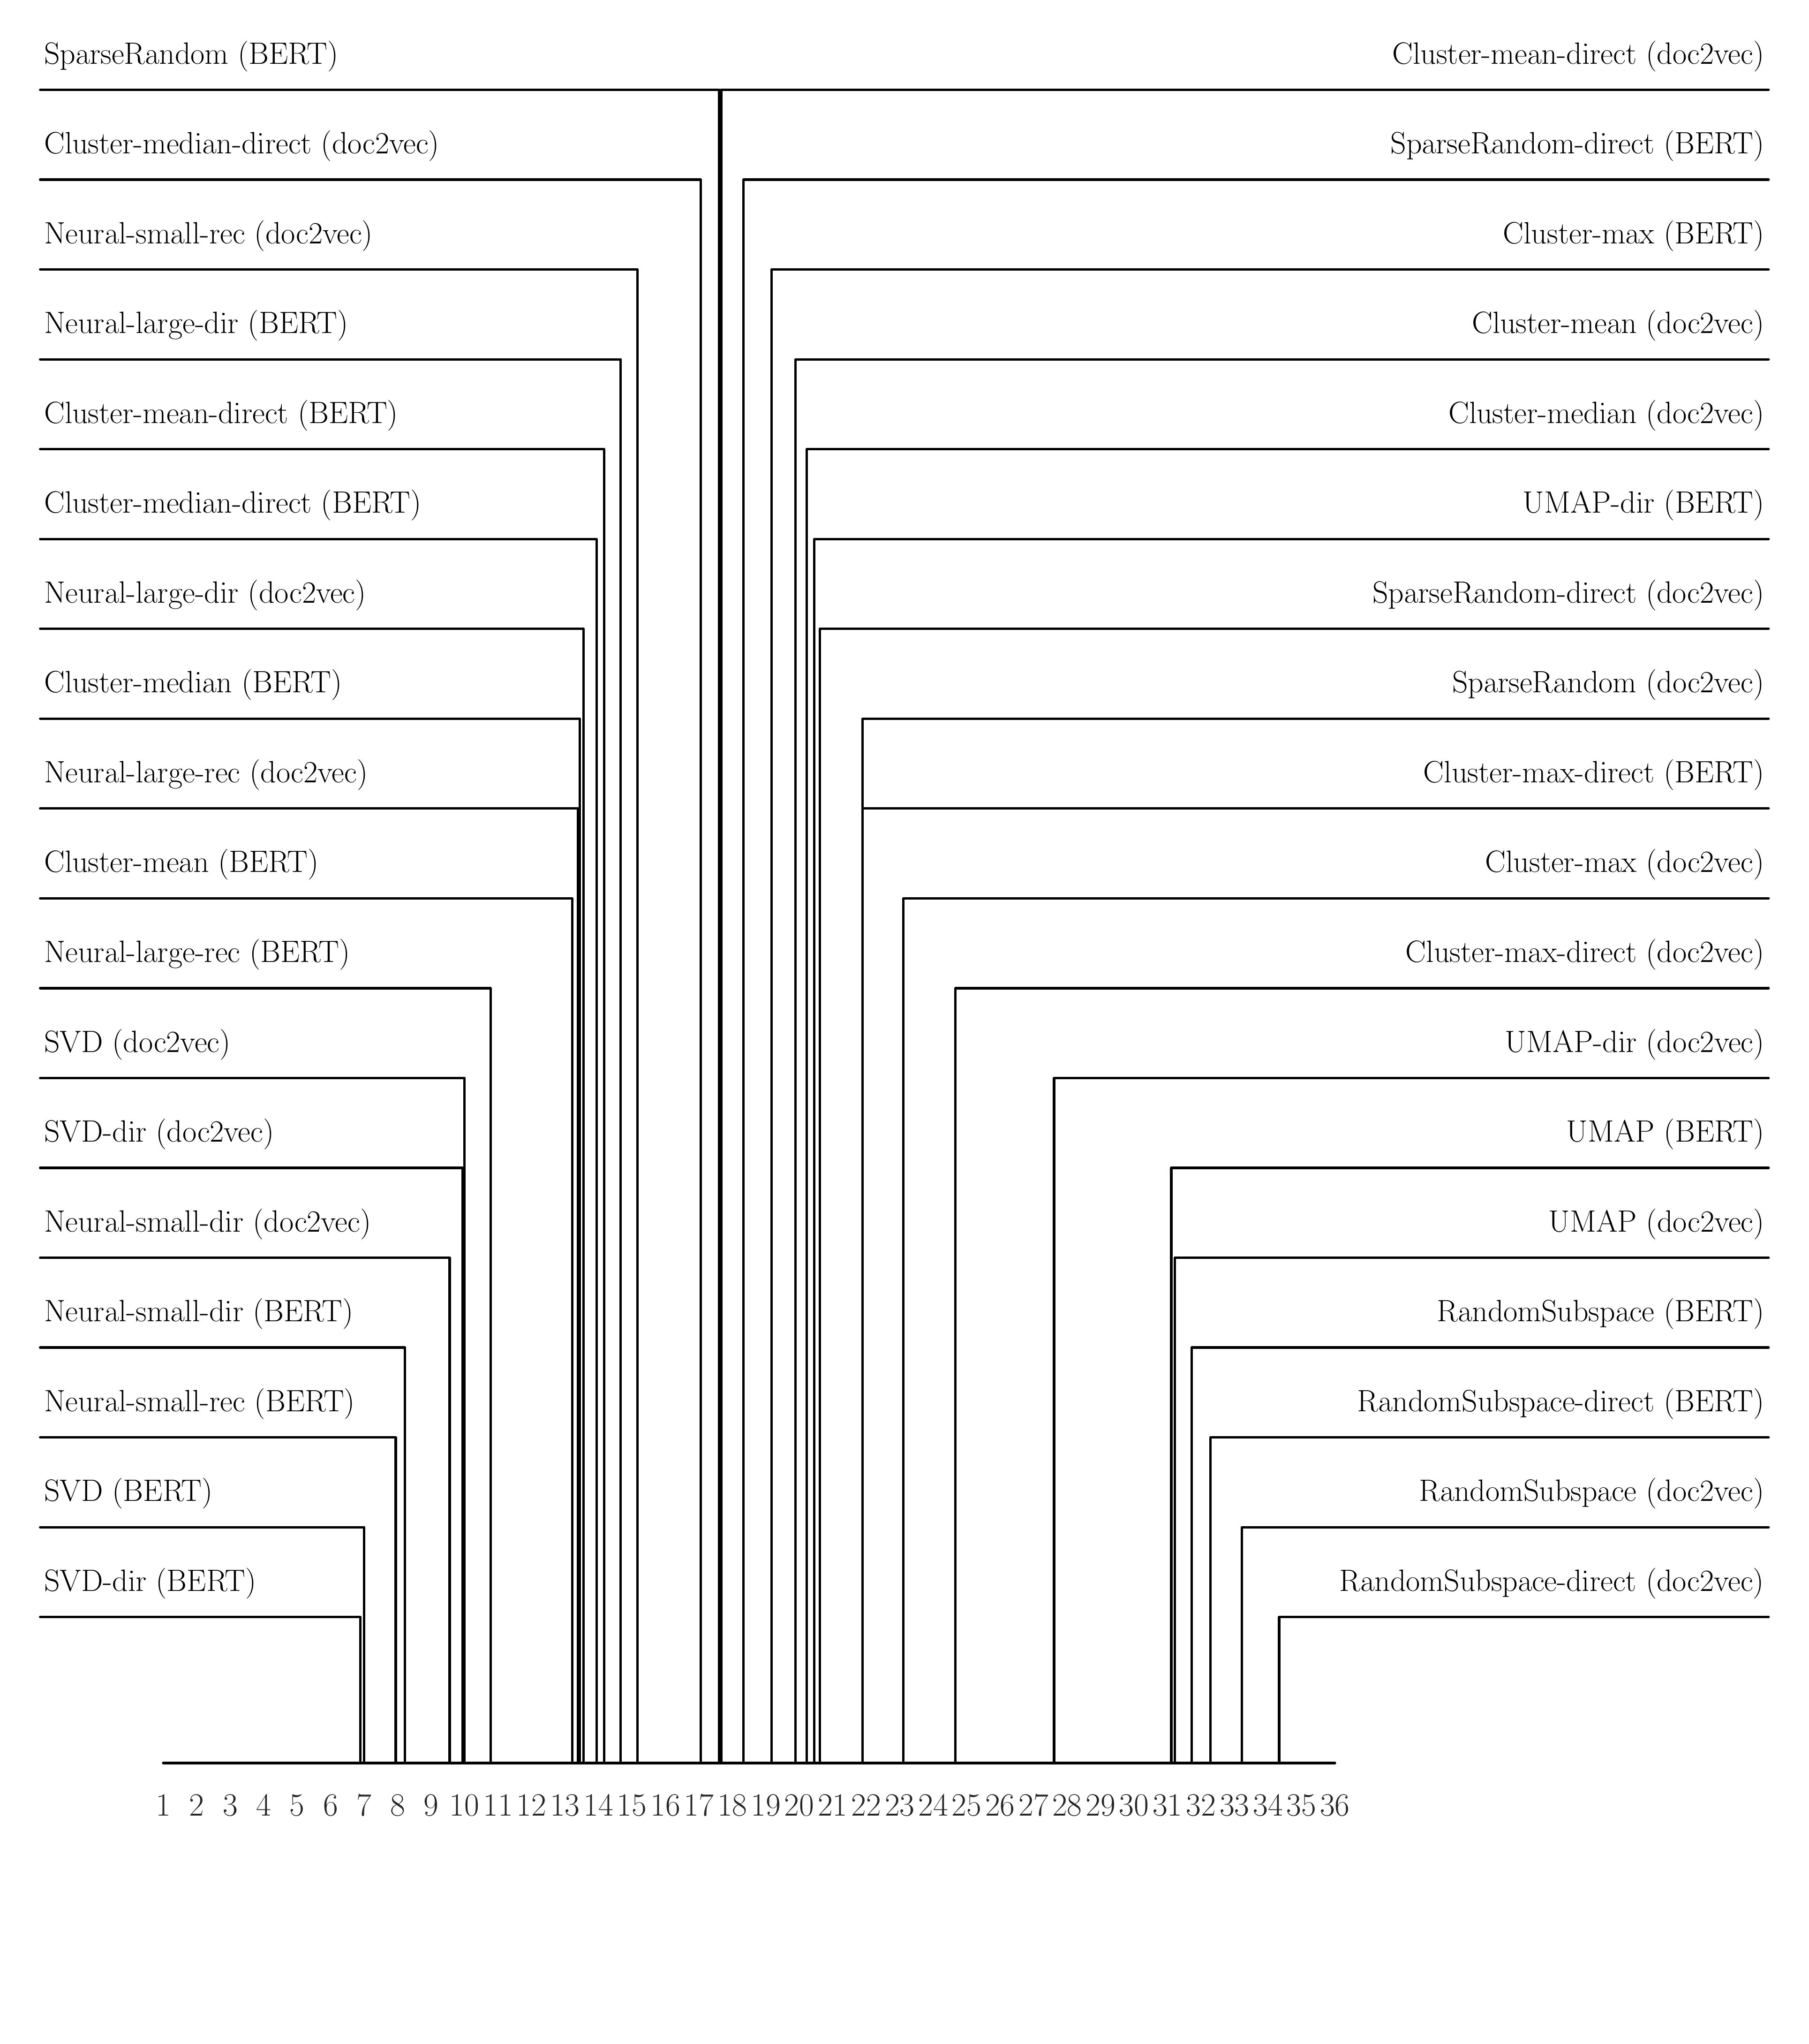}}
\caption{Critical distance diagrams of the representation-compressor pairs. It can be observed that recursive \emph{linear} representation performs well across different compression levels ($\tau$). When very high levels of compression are considered, however, the neural compression offers the best results. Note that the critical distance diagrams offer insight into the aggregation across all data sets, meaning that their interpretation needs to be in conjunction with the more detailed visualizations of performance in e.g., Figure 1.}
    \label{fig:cd}
\end{figure*}

\section{Other compression performances.}
In this section we present the compression performances, specific to each compression algorithm. It can be observed that most of the algorithm-representation pairs perform well on similar data sets.
\begin{table}[h!]
    \centering
    \begin{tabular}{llr}
\toprule
         Dataset & Compression step ($\kappa$) &  $\epsilon F1$ \\
\midrule
            mbti &               9 (dim = 2) &       0.002305 \\
         insults &               7 (dim = 6) &      -0.038501 \\
    pan-2017-age &               7 (dim = 6) &       0.128713 \\
         SMSSpam &              6 (dim = 12) &      -0.033070 \\
            yelp &              5 (dim = 24) &      -0.012800 \\
          kenyan &             2 (dim = 192) &      -0.034483 \\
        CNN-news &             1 (dim = 384) &      -0.045541 \\
        articles &             1 (dim = 384) &      -0.049420 \\
 MedicalRelation &             0 (dim = 768) &       0.000000 \\
         authors &             0 (dim = 768) &       0.000000 \\
 drugs-condition &             0 (dim = 768) &       0.000000 \\
       questions &             0 (dim = 768) &       0.000000 \\
         sarcasm &             0 (dim = 768) &       0.000000 \\
\bottomrule
\end{tabular}

    \caption{BERT - CoRe-large-dir}
    \label{}
\end{table}
\begin{table}[h!]
    \centering
    \begin{tabular}{llr}
\toprule
         Dataset & Compression step ($\kappa$) &  $\epsilon F1$ \\
\midrule
            mbti &               9 (dim = 2) &       0.002305 \\
         insults &               7 (dim = 6) &      -0.041540 \\
    pan-2017-age &               7 (dim = 6) &       0.089109 \\
         SMSSpam &              6 (dim = 12) &      -0.039540 \\
            yelp &              6 (dim = 12) &      -0.038800 \\
        CNN-news &             2 (dim = 192) &      -0.045541 \\
          kenyan &             2 (dim = 192) &      -0.043103 \\
 MedicalRelation &             1 (dim = 384) &      -0.047824 \\
        articles &             1 (dim = 384) &      -0.044218 \\
         authors &             0 (dim = 768) &       0.000000 \\
 drugs-condition &             0 (dim = 768) &       0.000000 \\
       questions &             0 (dim = 768) &       0.000000 \\
         sarcasm &             0 (dim = 768) &       0.000000 \\
\bottomrule
\end{tabular}

    \caption{BERT - CoRe-large-rec.}
    \label{}
\end{table}
\begin{table}[h!]
    \centering
    \begin{tabular}{llr}
\toprule
         Dataset & Compression step ($\kappa$) &  $\epsilon F1$ \\
\midrule
         insults &               9 (dim = 2) &      -0.041540 \\
            mbti &               9 (dim = 2) &       0.002766 \\
         SMSSpam &               7 (dim = 6) &      -0.030913 \\
    pan-2017-age &               7 (dim = 6) &       0.128713 \\
            yelp &               7 (dim = 6) &      -0.019600 \\
        CNN-news &              3 (dim = 96) &      -0.045541 \\
        articles &              3 (dim = 96) &      -0.043617 \\
 MedicalRelation &             2 (dim = 192) &      -0.036346 \\
          kenyan &             2 (dim = 192) &      -0.034483 \\
       questions &             2 (dim = 192) &      -0.049156 \\
         sarcasm &             2 (dim = 192) &      -0.040391 \\
         authors &             1 (dim = 384) &      -0.036513 \\
 drugs-condition &             1 (dim = 384) &      -0.033455 \\
\bottomrule
\end{tabular}

    \caption{BERT - CoRe-small-dir.}
    \label{}
\end{table}
\begin{table}[h!]
    \centering
    \begin{tabular}{llr}
\toprule
         Dataset & Compression step ($\kappa$) &  $\epsilon F1$ \\
\midrule
            mbti &               9 (dim = 2) &       0.000922 \\
    pan-2017-age &               7 (dim = 6) &       0.089109 \\
         SMSSpam &              6 (dim = 12) &      -0.026600 \\
         insults &              6 (dim = 12) &      -0.013171 \\
            yelp &              6 (dim = 12) &      -0.020400 \\
        CNN-news &              3 (dim = 96) &      -0.036053 \\
        articles &              3 (dim = 96) &      -0.044018 \\
 MedicalRelation &             2 (dim = 192) &      -0.043998 \\
          kenyan &             2 (dim = 192) &      -0.017241 \\
       questions &             2 (dim = 192) &      -0.046222 \\
         sarcasm &             2 (dim = 192) &      -0.043606 \\
         authors &             1 (dim = 384) &      -0.035618 \\
 drugs-condition &             1 (dim = 384) &      -0.032659 \\
\bottomrule
\end{tabular}

    \caption{BERT - CoRe-small-rec.}
    \label{}
\end{table}
\begin{table}[h!]
    \centering
    \begin{tabular}{llr}
\toprule
         Dataset & Compression step ($\kappa$) &  $\epsilon F1$ \\
\midrule
         insults &               9 (dim = 2) &      -0.042553 \\
            mbti &               9 (dim = 2) &       0.002305 \\
         SMSSpam &               7 (dim = 6) &      -0.040259 \\
    pan-2017-age &               7 (dim = 6) &       0.089109 \\
            yelp &               7 (dim = 6) &      -0.026800 \\
        CNN-news &              3 (dim = 96) &      -0.037951 \\
        articles &              3 (dim = 96) &      -0.046819 \\
          kenyan &              3 (dim = 96) &      -0.034483 \\
 MedicalRelation &             2 (dim = 192) &      -0.047824 \\
       questions &             2 (dim = 192) &      -0.044754 \\
         sarcasm &             2 (dim = 192) &      -0.042907 \\
         authors &             1 (dim = 384) &      -0.029732 \\
 drugs-condition &             1 (dim = 384) &      -0.023969 \\
\bottomrule
\end{tabular}

    \caption{BERT - PCA-dir.}
    \label{}
\end{table}
\begin{table}[h!]
    \centering
    \begin{tabular}{llr}
\toprule
         Dataset & Compression step ($\kappa$) &  $\epsilon F1$ \\
\midrule
         insults &               9 (dim = 2) &      -0.042553 \\
            mbti &               9 (dim = 2) &       0.002766 \\
         SMSSpam &               7 (dim = 6) &      -0.040259 \\
    pan-2017-age &               7 (dim = 6) &       0.089109 \\
            yelp &               7 (dim = 6) &      -0.025600 \\
        CNN-news &              3 (dim = 96) &      -0.045541 \\
        articles &              3 (dim = 96) &      -0.047219 \\
          kenyan &              3 (dim = 96) &      -0.034483 \\
 MedicalRelation &             2 (dim = 192) &      -0.043998 \\
       questions &             2 (dim = 192) &      -0.048423 \\
         sarcasm &             2 (dim = 192) &      -0.040391 \\
         authors &             1 (dim = 384) &      -0.029583 \\
 drugs-condition &             1 (dim = 384) &      -0.025957 \\
\bottomrule
\end{tabular}

    \caption{BERT - PCA-rec.}
    \label{}
\end{table}
\begin{table}[h!]
    \centering
    \begin{tabular}{llr}
\toprule
         Dataset & Compression step ($\kappa$) &  $\epsilon F1$ \\
\midrule
         SMSSpam &               9 (dim = 2) &      -0.036664 \\
         insults &               9 (dim = 2) &      -0.037487 \\
            mbti &               9 (dim = 2) &       0.002305 \\
    pan-2017-age &               7 (dim = 6) &       0.039604 \\
            yelp &              6 (dim = 12) &      -0.033600 \\
        CNN-news &             0 (dim = 768) &       0.000000 \\
 MedicalRelation &             0 (dim = 768) &       0.000000 \\
        articles &             0 (dim = 768) &       0.000000 \\
         authors &             0 (dim = 768) &       0.000000 \\
 drugs-condition &             0 (dim = 768) &       0.000000 \\
          kenyan &             0 (dim = 768) &       0.000000 \\
       questions &             0 (dim = 768) &       0.000000 \\
         sarcasm &             0 (dim = 768) &       0.000000 \\
\bottomrule
\end{tabular}

    \caption{BERT - UMAP-dir.}
    \label{}
\end{table}
\begin{table}[h!]
    \centering
    \begin{tabular}{llr}
\toprule
         Dataset & Compression step ($\kappa$) &  $\epsilon F1$ \\
\midrule
            mbti &               9 (dim = 2) &       0.002305 \\
    pan-2017-age &               7 (dim = 6) &       0.049505 \\
         SMSSpam &              3 (dim = 96) &      -0.030194 \\
         insults &             1 (dim = 384) &      -0.033435 \\
            yelp &             1 (dim = 384) &      -0.034800 \\
        CNN-news &             0 (dim = 768) &       0.000000 \\
 MedicalRelation &             0 (dim = 768) &       0.000000 \\
        articles &             0 (dim = 768) &       0.000000 \\
         authors &             0 (dim = 768) &       0.000000 \\
 drugs-condition &             0 (dim = 768) &       0.000000 \\
          kenyan &             0 (dim = 768) &       0.000000 \\
       questions &             0 (dim = 768) &       0.000000 \\
         sarcasm &             0 (dim = 768) &       0.000000 \\
\bottomrule
\end{tabular}

    \caption{BERT - UMAP-rec.}
    \label{}
\end{table}

\begin{table}[h!]
    \centering
    \begin{tabular}{llr}
\toprule
         Dataset & Compression step ($\kappa$) &  $\epsilon F1$ \\
\midrule
         insults &               9 (dim = 2) &      -0.020263 \\
         SMSSpam &               7 (dim = 6) &      -0.046010 \\
    pan-2017-age &               7 (dim = 6) &       0.079208 \\
        CNN-news &              6 (dim = 12) &       0.011385 \\
            yelp &              6 (dim = 12) &      -0.038400 \\
          kenyan &              5 (dim = 24) &      -0.008621 \\
       questions &              5 (dim = 24) &      -0.035950 \\
         sarcasm &              5 (dim = 24) &      -0.044864 \\
 MedicalRelation &              4 (dim = 48) &      -0.023912 \\
        articles &              4 (dim = 48) &      -0.035214 \\
            mbti &              4 (dim = 48) &       0.064085 \\
         authors &              3 (dim = 96) &      -0.036215 \\
 drugs-condition &             1 (dim = 384) &      -0.036238 \\
\bottomrule
\end{tabular}

    \caption{doc2vec - CoRe-large-dir}
    \label{}
\end{table}
\begin{table}[h!]
    \centering
    \begin{tabular}{llr}
\toprule
         Dataset & Compression step ($\kappa$) &  $\epsilon F1$ \\
\midrule
         insults &               9 (dim = 2) &      -0.014184 \\
    pan-2017-age &               7 (dim = 6) &       0.059406 \\
       questions &              6 (dim = 12) &       0.000734 \\
        CNN-news &              5 (dim = 24) &       0.039848 \\
         SMSSpam &              5 (dim = 24) &      -0.038821 \\
 MedicalRelation &              4 (dim = 48) &      -0.016260 \\
            mbti &              4 (dim = 48) &       0.012448 \\
         sarcasm &              4 (dim = 48) &      -0.028092 \\
            yelp &              4 (dim = 48) &      -0.036400 \\
        articles &              3 (dim = 96) &      -0.025010 \\
         authors &              3 (dim = 96) &      -0.040238 \\
          kenyan &              3 (dim = 96) &      -0.034483 \\
 drugs-condition &             1 (dim = 384) &      -0.034022 \\
\bottomrule
\end{tabular}

    \caption{doc2vec - CoRe-large-rec.}
    \label{}
\end{table}
\begin{table}[h!]
    \centering
    \begin{tabular}{llr}
\toprule
         Dataset & Compression step ($\kappa$) &  $\epsilon F1$ \\
\midrule
         insults &               9 (dim = 2) &      -0.017224 \\
         SMSSpam &               8 (dim = 3) &      -0.023005 \\
        CNN-news &               7 (dim = 6) &       0.032258 \\
    pan-2017-age &               7 (dim = 6) &       0.099010 \\
            yelp &               7 (dim = 6) &      -0.020800 \\
       questions &              6 (dim = 12) &      -0.046955 \\
         sarcasm &              6 (dim = 12) &      -0.041509 \\
 MedicalRelation &              5 (dim = 24) &      -0.043042 \\
        articles &              5 (dim = 24) &      -0.045018 \\
          kenyan &              5 (dim = 24) &      -0.043103 \\
            mbti &              5 (dim = 24) &       0.061319 \\
         authors &              4 (dim = 48) &      -0.046870 \\
 drugs-condition &             2 (dim = 192) &      -0.040100 \\
\bottomrule
\end{tabular}

    \caption{doc2vec - CoRe-small-dir.}
    \label{}
\end{table}
\begin{table}[h!]
    \centering
    \begin{tabular}{llr}
\toprule
         Dataset & Compression step ($\kappa$) &  $\epsilon F1$ \\
\midrule
         insults &               9 (dim = 2) &      -0.018237 \\
    pan-2017-age &               7 (dim = 6) &       0.059406 \\
       questions &               7 (dim = 6) &      -0.024945 \\
         SMSSpam &              6 (dim = 12) &      -0.023724 \\
        CNN-news &              5 (dim = 24) &       0.018975 \\
         sarcasm &              5 (dim = 24) &      -0.049755 \\
 MedicalRelation &              4 (dim = 48) &      -0.032520 \\
            mbti &              4 (dim = 48) &       0.002766 \\
            yelp &              4 (dim = 48) &      -0.023200 \\
        articles &              3 (dim = 96) &      -0.040216 \\
          kenyan &              3 (dim = 96) &      -0.008621 \\
 drugs-condition &             2 (dim = 192) &      -0.042770 \\
         authors &             1 (dim = 384) &      -0.020790 \\
\bottomrule
\end{tabular}

    \caption{doc2vec - CoRe-small-rec.}
    \label{}
\end{table}
\begin{table}[h!]
    \centering
    \begin{tabular}{llr}
\toprule
         Dataset & Compression step ($\kappa$) &  $\epsilon F1$ \\
\midrule
         insults &               9 (dim = 2) &      -0.022290 \\
         SMSSpam &               8 (dim = 3) &      -0.028037 \\
        CNN-news &               7 (dim = 6) &      -0.005693 \\
    pan-2017-age &               7 (dim = 6) &      -0.009901 \\
       questions &               7 (dim = 6) &      -0.044754 \\
          kenyan &              6 (dim = 12) &      -0.043103 \\
         sarcasm &              6 (dim = 12) &      -0.039413 \\
            yelp &              6 (dim = 12) &      -0.034800 \\
 MedicalRelation &              5 (dim = 24) &      -0.041129 \\
        articles &              5 (dim = 24) &      -0.043818 \\
            mbti &              5 (dim = 24) &       0.032273 \\
         authors &              3 (dim = 96) &      -0.021311 \\
 drugs-condition &             2 (dim = 192) &      -0.033171 \\
\bottomrule
\end{tabular}

    \caption{doc2vec - PCA-dir.}
    \label{}
\end{table}
\begin{table}[h!]
    \centering
    \begin{tabular}{llr}
\toprule
         Dataset & Compression step ($\kappa$) &  $\epsilon F1$ \\
\midrule
         SMSSpam &               9 (dim = 2) &      -0.036664 \\
         insults &               9 (dim = 2) &      -0.026342 \\
        CNN-news &               7 (dim = 6) &       0.005693 \\
    pan-2017-age &               7 (dim = 6) &       0.019802 \\
       questions &               7 (dim = 6) &      -0.026412 \\
         sarcasm &              6 (dim = 12) &      -0.040391 \\
            yelp &              6 (dim = 12) &      -0.026400 \\
 MedicalRelation &              5 (dim = 24) &      -0.047346 \\
        articles &              5 (dim = 24) &      -0.044218 \\
          kenyan &              5 (dim = 24) &      -0.043103 \\
            mbti &              5 (dim = 24) &       0.028124 \\
         authors &              4 (dim = 48) &      -0.049478 \\
 drugs-condition &             2 (dim = 192) &      -0.033625 \\
\bottomrule
\end{tabular}

    \caption{doc2vec - PCA-rec.}
    \label{}
\end{table}
\begin{table}[h!]
    \centering
    \begin{tabular}{llr}
\toprule
         Dataset & Compression step ($\kappa$) &  $\epsilon F1$ \\
\midrule
         SMSSpam &               9 (dim = 2) &       0.000000 \\
         insults &               8 (dim = 3) &      -0.021277 \\
    pan-2017-age &               7 (dim = 6) &       0.009901 \\
       questions &               7 (dim = 6) &      -0.026412 \\
 MedicalRelation &              4 (dim = 48) &      -0.042563 \\
        CNN-news &             0 (dim = 768) &       0.000000 \\
        articles &             0 (dim = 768) &       0.000000 \\
         authors &             0 (dim = 768) &       0.000000 \\
 drugs-condition &             0 (dim = 768) &       0.000000 \\
          kenyan &             0 (dim = 768) &       0.000000 \\
            mbti &             0 (dim = 768) &       0.000000 \\
         sarcasm &             0 (dim = 768) &       0.000000 \\
            yelp &             0 (dim = 768) &       0.000000 \\
\bottomrule
\end{tabular}

    \caption{doc2vec - UMAP-dir.}
    \label{}
\end{table}
\begin{table}[h!]
    \centering
    \begin{tabular}{llr}
\toprule
         Dataset & Compression step ($\kappa$) &  $\epsilon F1$ \\
\midrule
         insults &               9 (dim = 2) &      -0.018237 \\
    pan-2017-age &               7 (dim = 6) &       0.089109 \\
         SMSSpam &              3 (dim = 96) &      -0.000719 \\
       questions &              3 (dim = 96) &      -0.005869 \\
 MedicalRelation &             2 (dim = 192) &      -0.021043 \\
        CNN-news &             0 (dim = 768) &       0.000000 \\
        articles &             0 (dim = 768) &       0.000000 \\
         authors &             0 (dim = 768) &       0.000000 \\
 drugs-condition &             0 (dim = 768) &       0.000000 \\
          kenyan &             0 (dim = 768) &       0.000000 \\
            mbti &             0 (dim = 768) &       0.000000 \\
         sarcasm &             0 (dim = 768) &       0.000000 \\
            yelp &             0 (dim = 768) &       0.000000 \\
\bottomrule
\end{tabular}

    \caption{doc2vec - UMAP-rec.}
    \label{}
\end{table}

\bibliography{example_paper}
\bibliographystyle{icml2021}

\end{document}
